# Supplementary material for: An Empirical Study on Challenges of Event Management in Microservice Architectures
Source: arXiv:2408.00440 source file (2024-08-01)
Supplement: Supplementary file 1 [file 99_appendix.tex]

\appendix
